# Supplementary material for: How Important Is a Neuron?
Source: arXiv:1805.12233 source file (2018-05-30)
Supplement: Supplementary file 1 [file appendix.pdf]

---

# How Important Is a Hidden Unit? (Supplementary material)

---

Anonymous Author(s)

Affiliation

Address

email

## 1 Appendix

2 We illustrate the concept of conductance on a model that recognizes digits, i.e., the MNIST task.  
3 To illustrate the notion of conductance, we consider a simple convolutional neural network for  
4 digit recognition (MNIST). We use a network with two convolutional layers (with 32 and 64 filters  
5 respectively), two pooling layers, followed by two fully connected layers. We have computed  
6 conductances for filters in the first convolutional layer (32 filters) and displayed the top five filters for  
7 each input in Figure ?? . The figure shows both redundancy and some division of labour.

8 Another way to visualize the conductance is to compare the filters with most positive conductance to  
9 those with most negative conductance. Figure ?? compares the two sets of filters for the top predicted  
10 label for a given image. Notice that the filters with most negative conductance tend to focus on  
11 different parts of the image than the positive ones.

../Figures/mnist\_label\_0.jpeg

0.15 0.06 0.06 0.05 0.05

../Figures/mnist\_label\_1.jpeg

0.36 0.15 0.13 0.12 0.10

../Figures/ablation\_spaniel\_positive.jpeg

Filters with highest conductance for label = Welsh springer spaniel

../Figures/ablation\_spaniel\_negative.jpeg

Filters with most negative conductance for label = Welsh springer spaniel

../Figures/top\_filters\_africanelephant.jpeg

Label: African elephant    9.1       4.9       3.8

../Figures/top\_filters\_maltesedog.jpeg

Label: Maltese dog    4.2       3.9       2.8

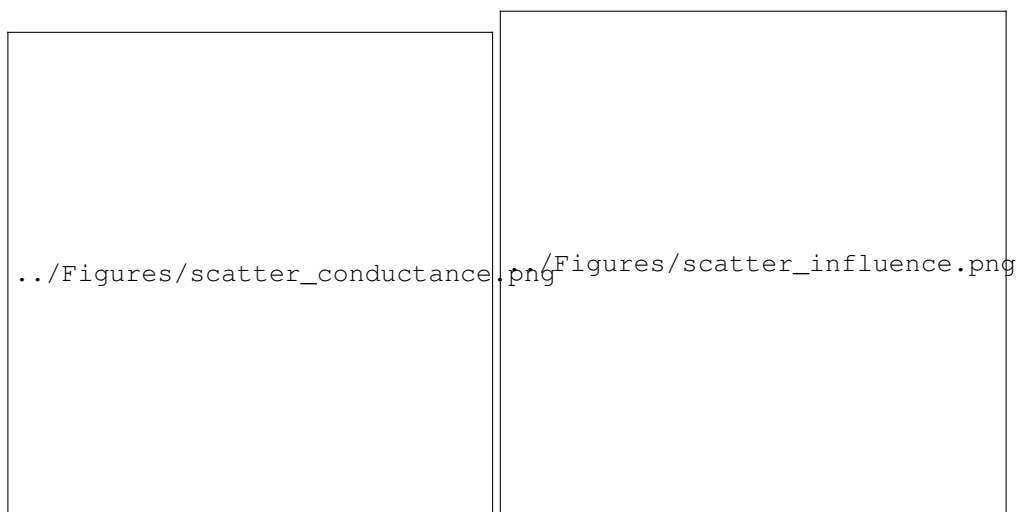

Figure 4: Left panel: conductance vs. ablation scores. Right Panel: internal influence vs. ablation scores. There is one data point per image, filter combination. Ablations scores show a stronger linear relation with the conductances.

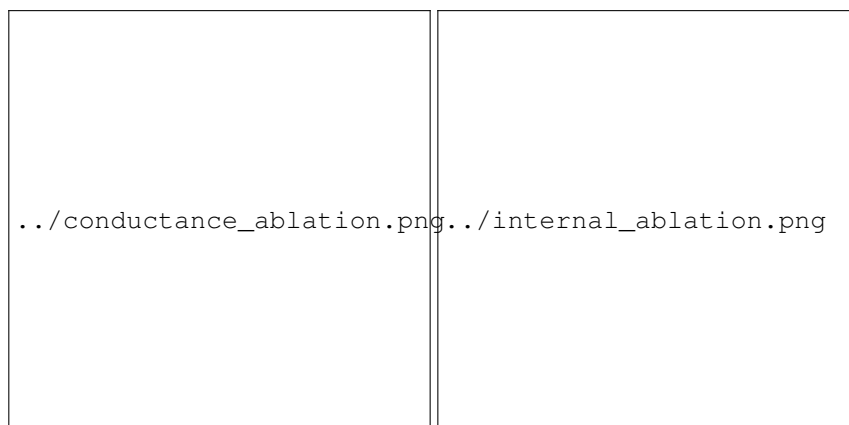

Figure 5: The first figure plots conductance vs. ablation scores. The second plots internal influence vs. ablation scores. There is one data point per example, filter combination. Notice the linear agreement in the first plot.
